# Supplementary material for: Cross-Link Channel Prediction for Massive IoT Networks
Source: arXiv:2212.07663 source file (2022-12-15)
Supplement: Supplementary file 1 [file appendix.tex]

\section{Scheduling and Resource Allocation Algorithm}
\label{s:sra}

\begin{algorithm}[t]
% \SetAlgoLined
\noindent 
\begin{algorithmic}[1] % enter the algorithmic environment
\Require 
    \Statex The up-to-date $CSI_{u}$ and $BSR_{u}$ $\forall u \in U$
\While{$\sum_{u}^{U} BSR_{u} > 0$}
    \State $MCS_{u}$ = \textbf{Rate-Adaptation}($CSI_{u}$) $\forall u \in U$
    \If{OFDMA}
        % Compute $MCS_{u}$ given $eSNR_{u}$ 
        \State Compute $R_{u} = BSR_{u}/T_{MaxTime}$ $\forall u \in U$
        \State Find $R_{RU(0)}, \dots, R_{RU(L)}$ given $MCS_{u}$ $\forall u \in U$
        \State $U_{l} \cap \left \{ u \right \}$ where  $l \geq \operatorname*{argmin}_{l \in L} \left \| R_{RU(l)} - R_{u} \right \| $
        \State $g_{opt} = \textbf{Divide-Conquer}(U, CSI, 0,0)$
    \Else
        \State $g_{opt} = \textbf{Greedy-Algorithm}(U, CSI,0,0)$
    \EndIf
    % \State Allocate $g_{RA} = g_{RU}-g_{SA}$ RUs for random access
    \While{empty $RU$ in $g_{opt}$}
        \State Pop $U_{l}$ if empty  $\forall l \in L$
        \State $g_{opt} = \textbf{Divide-Conquer}(U, CSI,0,0)$
    \EndWhile
    \State Set $T_{s} = max(min_{k \in g}(T_{k}), T_{MinTime})$
    % \If{Uplink}
    \State Transmit trigger frame
    % \EndIf
    \State Receive \text{scheduled-packet}
    \State $BSR_{u} = BSR_{u} - \text{Scheduled-Packet } \forall u \in g_{SA}$
    % \State Update $BSR_{u}~\forall u \in U$
    % \State 
\EndWhile
 \caption{Our SRA algorithm}
 \label{alg:general}
 \end{algorithmic} % enter the algorithmic environment
\end{algorithm}

\parahead{Our algorithm.}
%  the AP first sends a TF which
% now only indicates the ID of the group (i.e, the IDs of
% the scheduled users), and the dedicated sub-channel to each
% scheduled user. After receiving the TF, each user sends its
% buffer status (BS) information within the BS frame (i.e.,
% Qk(t)) by using its dedicated sub-channel. Also, the AP uses
% the BS frame to estimate the uplink transmission rate of user k
% (i.e., Rk(t)). Finally, the AP has both queue size and channel
% state information of each scheduled user at that time, and
% can determine the optimal scheduling duration denoted by $T_{s}$
Algorithm~\ref{alg:general} summarizes our SRA algorithm:
\textbf{(1)} we first find a proper MCS index for each user based on the acquired\fshyp{}predicted 
full\hyp{}bandwidth channel information.
To do so, we employ ESNR\hyp{}based
rate adaptation~\cite{halperin2010predictable}; 
\textbf{(2)} we then assign each user into one or more 
user groups $U_{0}, \dots , U_{L}$
% (\textit{e.g.} four groups for $20$~MHz
% as shown in Fig.~\ref{f:protocol:ru}) 
based on user's MCS index and BSR.
Here, high-level idea is to increase probability of users with low data rate to be assigned to smaller RUs while increasing likelihood of users with high data rate to be assigned to larger RUs.
Specifically, we first compute data-rate $R_{u}$ for each user $u$ via dividing user's buffer length by a maximum packet duration $T_{MaxTime}$, which is $5.484 ms$~\cite{802.11ax-wc16}. 
Then, we compare data-rate with predefined PHY rate~\cite{802.11ax-wc16} at the selected MCS index. 
If user's data rate $R_{u}$ is less than the predefined PHY rate $R_{RU(l)}$ at the level $l$ and selected MCS index,
we assign user $u$ to user groups $U_{l}, U_{l+1}, \dots, U_{L}$;
% in which among all levels whose $R_{RU}$ is greater than $R_{u}$, $R_{RU}$ is closest to the $R_{u}$. With this level $l$, we assign the users to all user groups whose level is greater than or equal to $l$.
\textbf{(3)} Given CSIs from all users and $L+1$ user groups, we run a divide\hyp{}conquer 
(DQ) algorithm~\cite{wang2018scheduling}.
Here, users can be allocated to RUs whose level $l$ corresponds with its assigned user group. 
For example, if user $u$ is assigned to user group $U_{2}$ and $U_{3}$ from step 2, then it can only be allocated to RUs with its size equivalent to level $2$ and $3$;
% However, if the protocol does not use OFDMA, then 
% predefined from step $2$; 
\textbf{(4)} if the schedule result in Step~$3$ contains RU with no assigned user, 
we repeat from Step~$2$ to rearrange users in $L+1$ user groups;
\textbf{(5)} finally, we set packet duration equal to the minimum duration among all scheduled users.
